# Supplementary material for: Efficient approximation for global functions of matrix product operators
Source: arXiv:1804.03613 source file (2018-04-13)
Supplement: Supplementary file 1 [file appendix.tex]

\section{Appendix Stuff}
\label{sec:appendix_stuff}
